# Supplementary material for: Coherent control of electron spin qubits in silicon using a global field
Source: arXiv:2107.14622 source file (2021-10-06)
Supplement: Supplementary file 1 [file Vahapoglu_et_al._Coherent_control_of_electron_spin_qubits_in_silicon_using_a_global_field_-_Supplementary_Information.pdf]

# Supplementary Information: Coherent control of electron spin qubits in silicon using a global field

E. Vahapoglu[1], J. P. Slack-Smith[1], R. C. C. Leon[1], W. H. Lim[1], F. E. Hudson[1], T. Day[1], J. D. Cifuentes[1], T. Tanttu[1], C. H. Yang[1], A. Saraiva[1], N. V. Abrosimov[2], H.-J. Pohl[3], M. L. W. Thewalt[4], A. Laucht[1], A. S. Dzurak[1,*], and J. J. Pla[1,*]

[1] *School of Electrical Engineering and Telecommunications, UNSW Sydney, Sydney, NSW 2052, Australia.*
[2] *Leibniz-Institut für Kristallzüchtung, 12489 Berlin, Germany.*
[3] *VITCON Projectconsult GmbH, 07745 Jena, Germany.*
[4] *Department of Physics, Simon Fraser University, Burnaby, British Columbia V5A 1S6, Canada.*
[*] *These authors contributed equally to this work*

# I Experimental Setup and Qubit Device

The setup used in this work is similar to the one in Ref. [1], with additional attenuation on the microwave line to protect the device from room temperature noise (See Fig. S1).

The device in this work has a gate layout that replicates the one used in Ref. [1] (See SEM in Fig. S2). However, it also includes an unused (floating) microwave transmission line (TL)[2] in the vicinity of the quantum dots, which is fabricated for conventional TL-based ESR measurements.

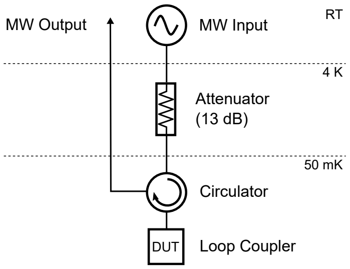


**Figure S1: Microwave control setup diagram.** Schematic of the microwave components used in the experiment.

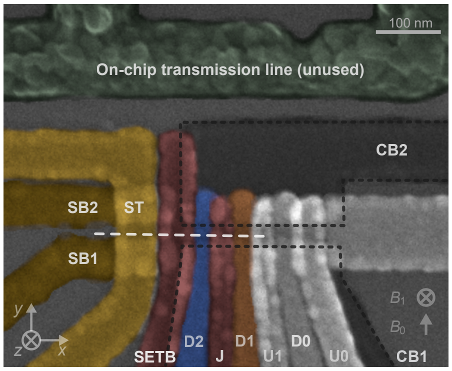


**Figure S2: Device SEM image.** A false colored scanning electron microscope (SEM) image of a device identical to the one measured in this work. Gates U1 and U0 are unused in our experiments.

# II Electric Field Generated by the Dielectric Resonator

We indirectly probe the electric field produced by the microwave signal sent to the loop coupler through an experiment where we monitor several Coulomb peaks of the SET with the microwave signal on.

We first perform a sweep of the microwave power with the frequency selected to be on-resonance with the DR (Fig. S3a and c). Even though a slight broadening is observed for powers as low as -45 dBm, the peaks are still resolved at -28 dBm where we have observed coherent control (see Fig. 2 of the main text).

In order to investigate if the DR enhances the electric field, we also sweep the MW frequency (Fig. S3b and d) at a fixed power over a range that covers the DR resonance. There is no evidence of an enhanced electric field within the DR resonance, where the Coulomb peak width appears to reduce slightly.

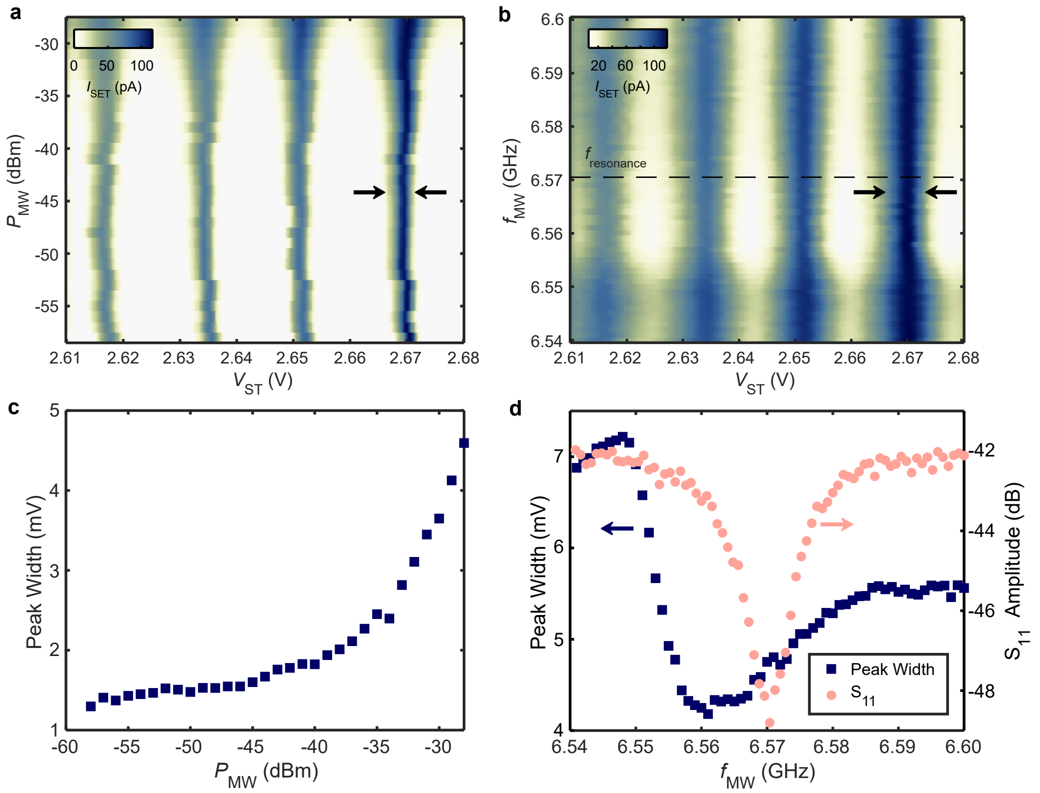


**Figure S3: SET Coulomb peaks vs MW power and frequency.** SET Coulomb peaks measured as a function of an always-on microwave signal applied to the loop coupler, **a**, Coulomb peaks vs. microwave power with $f_{\mathrm{MW}} = f_{\mathrm{resonance}} = 6.5705$ GHz. **b**, Coulomb peaks vs. microwave frequency with $P_{\mathrm{MW}} = -30$ dBm. **c-d**, Fitted peak width of the peaks marked with black arrows in panels a and b, respectively. The DR $S_{11}$ has been superimposed on panel d.

# III Extended Charge Stability Map

To further support our conclusion on the number of electrons in our double dot system, we provide a charge stability map taken over a larger range of J gate voltages in Fig. S4 than the one in the main text (Fig. 1d). The number of transitions remain the same for a $V_J$ range of 0.3V. The transitions become less visible at lower $V_J$, as the tunnel rates reduce below twice the AC excitation frequency (487 Hz), indicating that the J gate is successful in tuning the tunnel coupling between the dots.

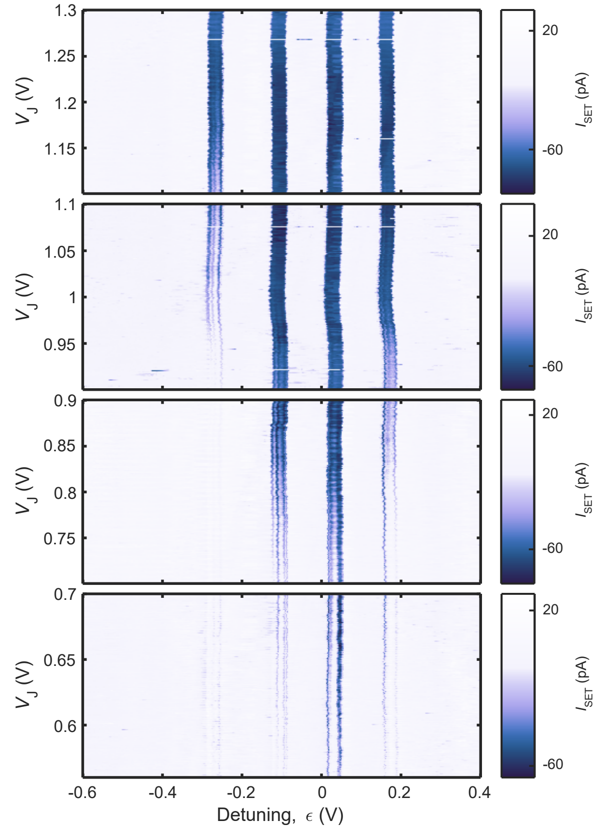


**Figure S4: Charge Stability Map.** An expanded version of the stability map in Fig. 1d with a larger J gate voltage range.

## IV Singlet State Initialization

The energy diagram in Fig. S5 visualizes how we initialize the two-spin system as singlet for all of the ESR measurements in this work. We first wait for 200 $\mu$s in the voltage configuration indicated by the 'circle', which is somewhere in the (4,0) charge region, to prepare a singlet state with two electrons in the same dot. The remaining two electrons are in a lower orbital state, forming a closed shell and do not interact with the other pair. We then diabatically ramp to the point marked by the 'star' in (3,1), which moves one electron to the other dot, while protecting the singlet state. Due to the nonzero g-factor difference of the electrons on either dot, the singlet state in (3,1) quickly decays to $|\downarrow\uparrow\rangle$, resulting in two slightly different ESR frequencies.

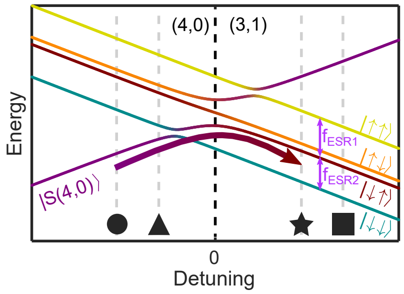


**Figure S5: Energy diagram.** A schematic energy diagram depicting the energy levels of the eigenstates in the measured double dot system with respect to voltage detuning. The vertical black dashed line is where the charge transition occurs. The detuning points marked with black geometric shapes are the same as the voltage configurations in Fig. 1d and e of the main text. The curved arrow with color gradient shows how the singlet state is initialized.

# V Stark Shift Measurements

In order to identify the location of each qubit with respect to the gates, we measure the Stark shift effect that results from changing the potentials on the plunger gates D0, D1 and D2 (see Fig. S6). The ESR frequency of Qubit 1 is mostly sensitive to D1, even though it is also affected by D0 and D2. As for Qubit 2, only the D2 gate has an observable effect on its frequency. These results indicate that Qubit 1 and 2 most likely reside under D1 and D2, respectively.

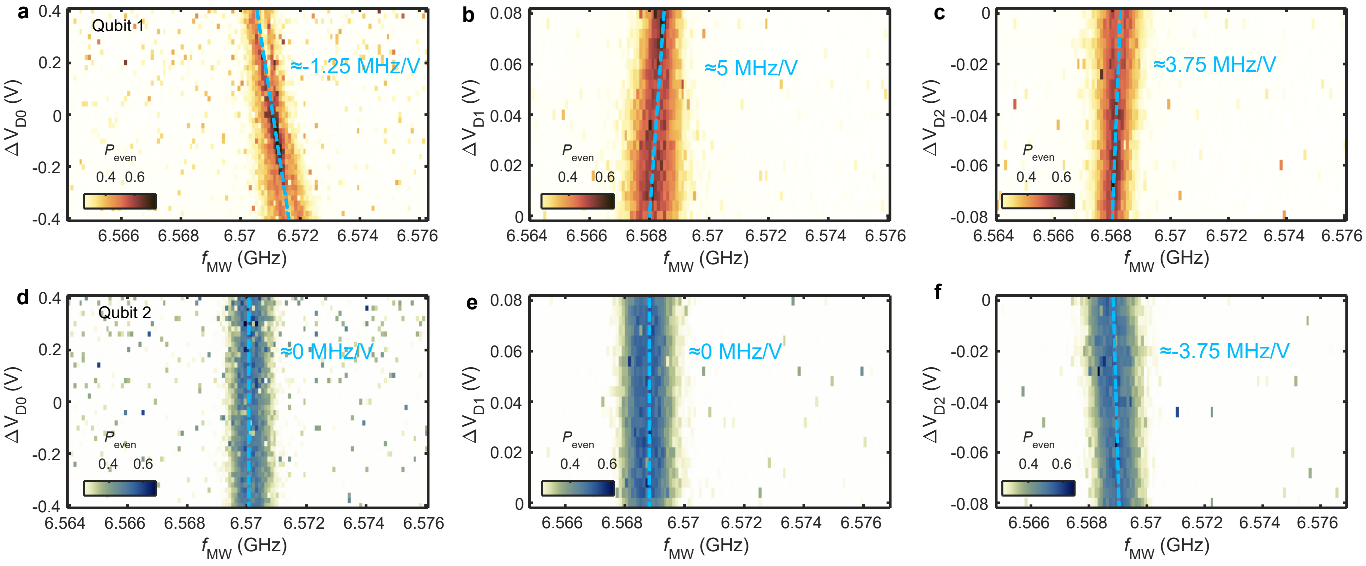


**Figure S6: Stark shift measurements**. $P_{\mathrm{even}}$ measured as a function of $f_{\mathrm{MW}}$ and the DC voltages applied to plunger gates D0-D2 for Qubit 1 (**a-c**) and Qubit 2 (**d-f**). The light blue dashed lines serve as guides showing how the ESR frequencies change with respect to the gate voltages. The numbers next to the lines correspond to approximate Stark shift values. The DC magnetic field $B_0$ is applied in the [110] crystallographic direction and has a magnitude of 241 mT, whereas the MW field generated by the DR is along [001].

# References


[1] Vahapoglu, E. *et al.* Single-electron spin resonance in a nanoelectronic device using a global field. *Science Advances* **7**, eabg9158 (2021).

[2] Dehollain, J. P. *et al.* Nanoscale broadband transmission lines for spin qubit control. *Nanotechnology* **24**, 015202 (2013).
